# Supplementary material for: MV-Map: Offboard HD-Map Generation with Multi-view Consistency
Source: arXiv:2305.08851 source file (2023-10-09)
Supplement: Supplementary file 2 [file hdmapnet.tex]

\begin{table}[tb]
\caption{MV-Map generalizes to other onboard models. Using HDMapNet~\cite{li2022hdmapnet} with both camera and LiDAR modalities as our onboard model, \ourmodel is consistently effective and significantly improves the HD-Map quality. We evaluate under the same short-range setting as HDMapNet.} \vspace{-2mm}
    \centering
    \resizebox{0.99\linewidth}{!}{
    \begin{tabular}{c|cccc}
    \toprule
    \multirow{2}{*}{\ourmodel} & 
    \multicolumn{4}{c}{mIoU (Short-range)} \\ & Divider & Ped Crossing & Boundary & All   \\ 
    \midrule
    \xmark & 46.20  & 24.38  & 56.99 & 42.52 \\
    \cmark & \textbf{49.82}  & \textbf{29.83}  & \textbf{58.54} & \textbf{46.06} \\
    \bottomrule
    \end{tabular}
    }
    
    \vspace{-2mm}
    \label{tb:supp-encoder-hdmapnet}
\end{table}
